# Supplementary material for: Shaping non-reciprocal caustic spin-wave beams
Source: arXiv:2404.15011 source file (2026-02-11)
Supplement: Supplementary file 1 [file SOM_ShapingCausticBeam_V2.pdf]

# Supplementary Materials: Shaping non-reciprocal caustic spin-wave beams

Dinesh Wagle,[1] Daniel Stoeffler,[2] Loic Temdie,[3] Mojtaba Taghipour Kaffash,[1] Vincent Castel,[3] Hicham Majjad,[2] Romain Bernard,[2] Yves Henry,[2] Matthieu Bailleul,[2] M. Benjamin Jungfleisch,[1,*] and Vincent Vlaminck[3,†]

[1]*Department of Physics and Astronomy, University of Delaware, Newark, DE 19716, USA*

[2]*IPCMS - UMR 7504 CNRS Institut de Physique et Chimie des Materiaux de Strasbourg, France*

[3]*IMT- Atlantique, Dpt. MO, Lab-STICC - UMR 6285 CNRS, Technopole Brest-Iroise CS83818, 29238 Brest Cedex 03, France*

(Dated: December 19, 2024)

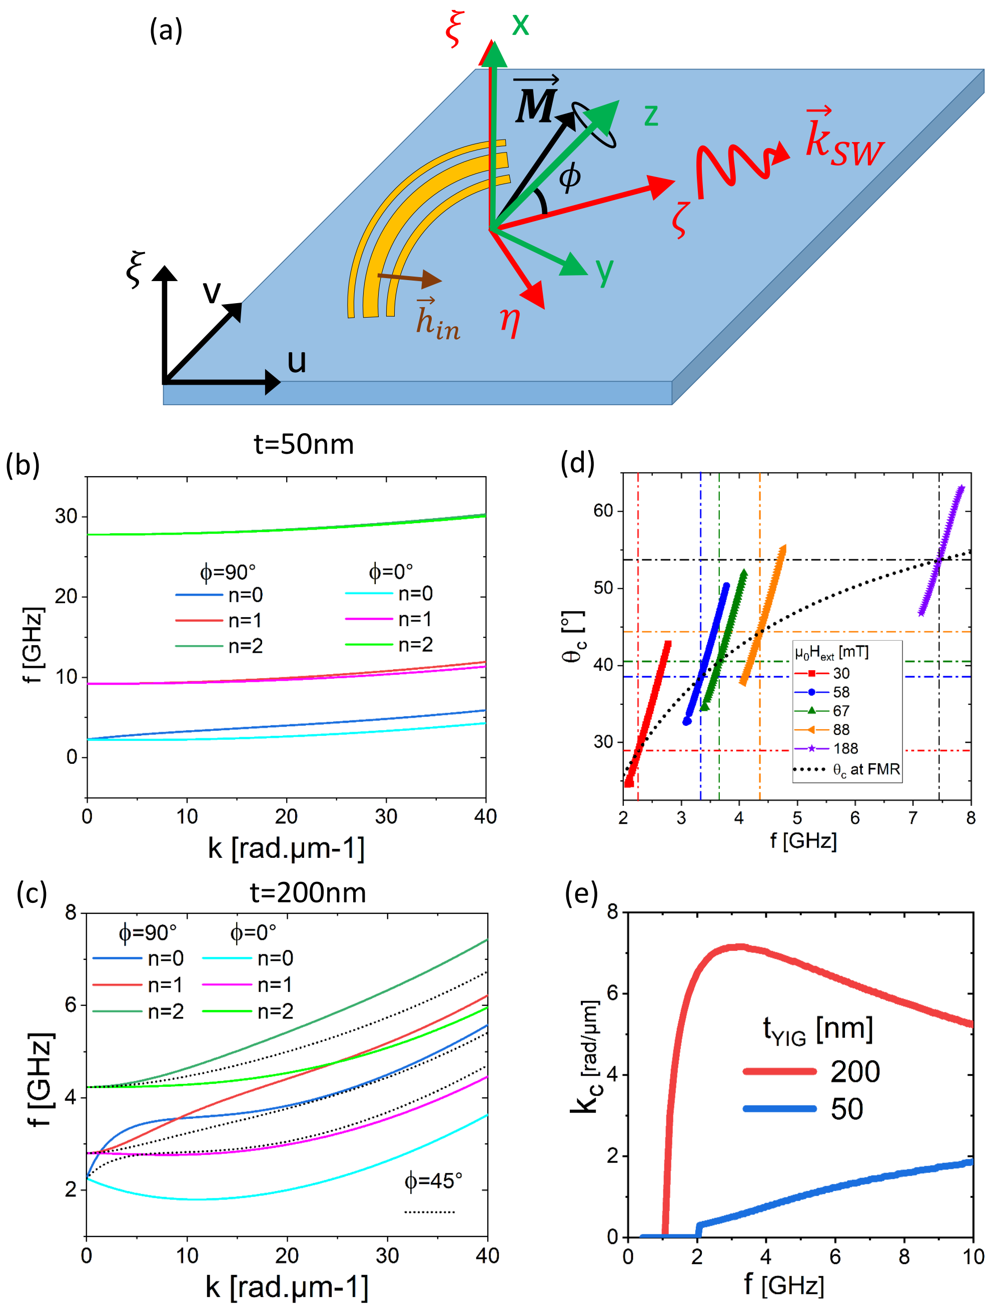


Supplementary Fig. 1. (**a**) Sketch of the geometry for the near-field diffraction model for in-plane mode showing the three frames of reference ($u$,$v$,$\xi$), ($x$,$y$,$z$), and ($\xi$,$\eta$,$\zeta$). (**b**) and (**c**) Dispersion relations for the first 3 thickness modes with $\phi = 0°$ and $90°$ at $\mu_0 H_{ext}$=30 mT, respectively for (**b**) a 50 nm-thick, and (**c**) 200 nm-thick YIG film (dotted lines are the dispersion relation at $\phi = 0°$). (**d**) Frequency dependence of the caustic angle for a 200nm-thick YIG film. (**e**) Frequency dependence of the caustics wavevector $k_c$ when the field is chosen to meet FMR conditions.

# I. NEAR-FIELD DIFFRACTION MODEL FOR IN-PLANE MAGNETIZED THIN FILM

We present step-by-step the near-field diffraction approach adapted to in-plane magnetized films, which requires the linear dynamic susceptibility tensor $\chi(k_u,k_v)$ in order to calculate the dynamic magnetization transverse to the equilibrium direction $\vec{m}(u,v)=(m_{in},m_{out})$ for a given excitation profile $\vec{h}(k_u,k_v)=(h_{in},h_{out})$, where the index $in$ (resp. $out$) refers to the in-plane (resp. out-of-plane) components. Our model is an extension of Eq. (34) of Kalinikos's seminal work [1] to the more general case of a 2D-shaped antennas:

$$\vec{m}(u,v,t) = e^{i\omega t} \iint_{-\infty}^{+\infty} dk_u dk_v \chi(k_u,k_v) \vec{h}(k_u,k_v) e^{-i(k_u u + k_v v)}. \tag{1}$$

Following their approach, we define three frames of reference as sketched in Supplementary Fig. 1-(a). Firstly, we define the reference frame of the lab ($u$,$v$,$\xi$) based on the orientation and/or symmetry of the spin-wave antenna, where $\xi$ is the coordinate normal to the film plane. Secondly, we define the frame ($x$,$y$,$z$) in which we linearize the Landau-Lifschitz-Gilbert (LLG) equation. This reference frame is defined such that the static equilibrium magnetization points in the $z$-direction, and the $x$-coordinate coincides with $\xi$. In this second reference frame, the dynamic part of the linearized LLG equation accounting for the exchange and dipolar dynamic fields can be written as:

$$\vec{h} = \left( \begin{pmatrix} 0 & -1 \\ 1 & 0 \end{pmatrix} i\frac{\omega}{\omega_M} + (\Omega_k + i\alpha\frac{\omega}{\omega_M})\mathbb{I} + \mathbb{N}_{ij}^{(0,0)} \right) \vec{m}, \tag{2}$$

where $\vec{h}$ is the excitation field from an antenna with arbitrary spatial distribution in the 2D plane, $\omega_M = \gamma\mu_0 M_s$, $\Omega_k = \frac{\gamma\mu_0 H_{equ}}{\omega_M} + \Lambda^2 k^2$ with $\Lambda^2 = \dfrac{2A_x}{\mu_0 M s^2}$ the exchange length, $\mathbb{I}$ the identity matrix, and $\mathbb{N}_{ij}$ the dynamic demagnetizing tensor. Lastly, in order to explicit the dynamic demagnetizing tensor, we define a frame related to the spin-wave propagation ($\xi$,$\eta$,$\zeta$), such that $\zeta$ is the propagation direction of an elementary spin wave. In this frame, the dynamic dipolar field $\vec{h_d} = -\mathbb{N}_{ij}\vec{m}$ for each combination of spin-wave modes $(n_1,n_2)$ written in the set of plane waves with standing wave profile across the thickness $t$ is given by [2]:

$$\mathbb{N}_{ij}^{(n_1,n_2)} = -\iint_{-t/2}^{t/2} d\xi\, d\xi'\, m_{j,n_2}\, \mathbb{G}_{ij}(\xi-\xi')\, m_{i,n_1}, \tag{3}$$


* mbj@udel.edu

† vincent.vlaminck@imt-atlantique.fr

where $\mathbb{G}_{ij}$ is the Green function tensor, which in the ($\xi$,$\eta$,$\zeta$) frame is defined as:

$$\mathbb{G}_{ij}(\xi-\xi') = \begin{pmatrix} G_P - \delta(\xi-\xi') & 0 & iG_Q \\ 0 & 0 & 0 \\ iG_Q & 0 & -G_P \end{pmatrix} \quad (4)$$

with $G_P = \frac{k}{2}e^{-k|\xi-\xi'|}$ and $G_Q = sign(\xi-\xi')G_P$. For simplicity, we will only consider the fundamental mode ($n = 0$) that has a uniform amplitude across the thickness, and use unpinned conditions at both interfaces ($\left(\frac{\partial \vec{m}}{\partial z}\right)_{\pm t/2} = \vec{0}$). In this case, the demagnetizing tensor expressed in the ($x$,$y$,$z$) frame takes the form:

$$\mathbb{G}_{ij}(\xi-\xi') = \begin{pmatrix} 1-P & 0 \\ 0 & P\sin^2(\phi) \end{pmatrix}, \quad (5)$$

where $P = -\frac{1}{t}\iint_{-t/2}^{t/2} d\xi\, d\xi' G_P(\xi-\xi') = 1 - \frac{1-e^{-kt}}{kt}$, and $\phi$ is the angle between the magnetization and the wavevector.

Next, the susceptibility tensor in reciprocal space $\chi(k_x, k_y)$ is obtained by inverting Eq. (2):

$$\chi_{ij} = \frac{1}{|\chi^{-1}|} \begin{pmatrix} \Omega_k + i\alpha\dfrac{\omega}{\omega_M} + P\sin^2(\phi) & i\dfrac{\omega}{\omega_M} \\ -i\dfrac{\omega}{\omega_M} & \Omega_k + i\alpha\dfrac{\omega}{\omega_M} + 1 - P \end{pmatrix}, \quad (6)$$

with the determinant of the system $|\chi^{-1}| = \frac{1}{\omega_M^2}(\omega_{res}^2 - \omega^2 + i\alpha\omega(2\Omega_k + \omega_M(1 - P\cos^2(\phi)))$, and $\omega_{res}$ is the dispersion relation for the $n = 0$ mode [3]:

$$\omega_{res}^2(k, H, \phi) = \Omega_k\omega_M^2(\Omega_k + (1 - P\cos^2(\phi) + \frac{(1-P)P\sin^2(\phi)}{\Omega_k})), \quad (7)$$

where $H$ is the static bias field, $P = 1 - \dfrac{1-e^{-kt}}{kt}$, $t$ is the film thickness, $k = \sqrt{k_u^2 + k_v^2}$, $\omega_M = \gamma\mu_0 M_s$, $\Omega_k = \frac{\gamma\mu_0 H_{equ}}{\omega_M} + \Lambda^2 k^2$ with $H_{equ}$ the equilibrium field including possible anisotropy, $\Lambda^2 = \dfrac{2A_x}{\mu_0 M s^2}$ the exchange length, and $\phi$ is the angle between the equilibrium magnetization and the wavevector.

Restricting ourselves to just the fundamental mode somewhat limits the validity of our model to sufficiently thin films because we do not account for a spin-wave amplitude across the film thickness. We believe that expanding the linear system with higher order modes up to a sufficient order $n$, including the coupling between the different modes, would allow us to recover the thickness dependence of the interference patterns. Adding this expansion would

make the model significantly more complicated, which in its current form yields accurate results for sufficiently thin films ($t$ $\leq$50 nm). Besides, the dirsperions relations shown in Supplementary Fig. 1-(b),(c) show that the higher order modes are fairly decoupled for a 50 nm thick film, whereas in the 200 nm thick film, mode crossing for the first two modes may occur in the range of wavevectors and angle $\phi$ where caustics are effectively excited (cf Supplementary Fig. 1-(d)). We present the frequency dependence of the caustic wavevector in Supplementary Fig. 1-(e), while fixing the field to the FMR conditions for each frequency. The identification of the caustic point was done using the dispersion relation as follow: Firstly, we define a set of values for $k_v$ and find with a root-finding method the corresponding $k_u$ value to plot the isofrequency. Secondly, we compute numerically the first and second order derivative ($dk_v/dk_u$ and $d^2k_v/dk_{u^2}$). Finally, starting from the highest value of $k_v$ , we search for a sign change in the second derivative to identify the caustic point. We can identify a cut-off frequency around 900 MHz for the existence of caustic formation, and see that the evolution of the caustic wavevector is non-monotonous over the frequency range with a maximum value of 7.75 rad.$\mu$m$^{-1}$ at around 3 GHz for the 200nm-thick film. For the 50 nm-thick film, the cut-off frequency is higher (at 2 GHz), and the frequency dependence of the caustic wavevector appears monotoneous.

Then, we resort to the last change of the frame to express the dynamic susceptibility tensor in the Lab frame ($u$,$v$,$\xi$), and perform the matrix product with the microwave field $\vec{h}(k_u,k_v)$=$(h_{in}, h_{out})$. Finally, we compute the inverse Fourier transform of each component of the product to obtain the mappings of the dynamic components of the magnetization $\vec{m}(u, v)$=$(m_{in}, m_{out})$. For the FFT of the NFD simulations, we directly implemented the routine from NUMERICAL RECIPES IN C [4], which requires a power of 2 number of points in each coordinate (e.g. a total of $N = 2^K * 2^K$ points). In order to avoid artifacts due to reflections at the edges, we typically resort to at least K=12 (N= 16777216) with a stepsize of 50nm, which corresponds to a window size of 200*200 $\mu$m$^2$ sufficiently large to have vanishing amplitudes.

We compare in Supplementary Fig. 2 the spin-wave diffraction patterns obtained respectively for a 5 $\mu$m segment, and a 500 nm square segment on top of a 50 nm YIG film using $\mu_0 M_s$=181.4 mT, no anisotropy, a gyromagnetic ratio $\gamma$=28.2 GHz.T$^{-1}$, an exchange constant of $A_x$=4 pJ/m, and a Gilbert damping $\alpha = 2 \times 10^{-4}$. In these simulations, we defined

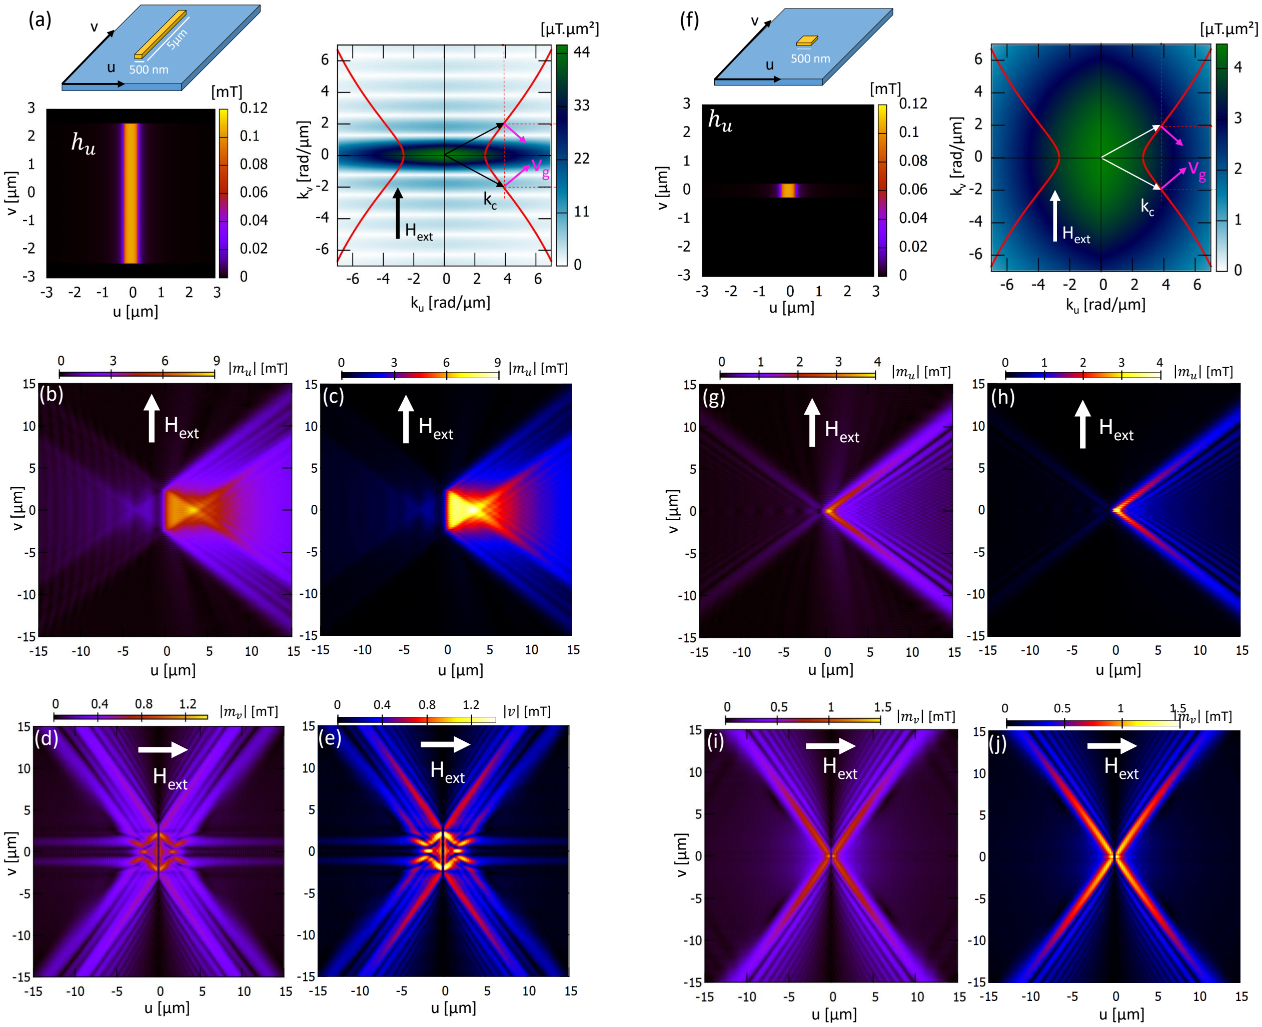


Supplementary Fig. 2. (**a**) Excitation profile and isofrequency curve at 7.9 GHz for a 50 nm thick YIG film magnetized along $v$-axis under a bias field of 200mT, superimposed with the Fourier transform of the excitation field from a 5 $\mu$m long segment and (**f**) a 500 nm square. (**b**) NFD, (**c**) MuMax3 simulations in the DE-configuration, and (**d**) NFD, (**e**) MuMax3 simulations in the BVW configuration for the 5 $\mu$m-long segment. (**g**)Corresponding NFD, (**h**), MuMax3 simulations in the DE-configuration, and (**i**) NFD, (**j**) MuMax3 simulations in the BVW configuration for the 500 nm square.

the excitation profile from the expressions of the Oersted field for a 80 nm-thick straight rectangular conductor carrying uniform current density along $v$, and adjusting the current value to limit a maximum field value of 0.1 mT. In all NFD simulations, we represented the modulus quantity $|m_{in}|(u, v) = \sqrt{Re(m_{in})^2 + Im(m_{in})^2}$ of in-plane component $m_{in}$ of the

dynamic magnetization in Eq.(1) of the article. We simulated two limiting cases: (1) when the bias field is perpendicular to the in-plane dynamic field [Supplementary Figs. 2(b,g), "Damon-Eshbach"-like configuration (DE)], and (2) when the bias field is parallel to the in-plane dynamic field [Supplementary Figs. 2(d,i), "backward volume wave"-like configuration (BVW)]. Alongside the NFD mapping, we also show in Supplementary Figs. 2(c,h,e,j) the corresponding micromagnetic simulations performed with MuMax3 using the same set of parameters, and the same excitation profile. We used a 41.6*41.6 $\mu$m$^2$ window discretized in $(16.6)^3$ nm$^3$ cells having a 6.7 microm large absorbing contour within which the Gilbert damping increases gradually to 0.1 in order to avoid reflections. All MuMax3 simulations show the steady state amplitude of the dynamic magnetization. We adopted a $sin(2\pi\, f\, t)$ excitation, and recorded the spatial and temporal evolution of the dynamic magnetization $m(u, v, t) = |m_{in}(u, v)| sin(2\pi\, f\, t + \Phi(u, v))$ for each pixel over a full period $T = 1/f$ after the steady state had been reached, which typically takes about $1000 * T$ to occur. One can clearly appreciate the excellent quantitative comparison between both methods in the smallest details of the diffraction pattern. Recalling that the computing ressources needed for a NFD mapping are negligible in comparison with its corresponding micromagnetic simulation, these simple tests validate the NFD approach for sufficiently thin in-plane magnetized films and highlight its suitability to explore magnon beam-forming and magnon interferometry in the linear regime.

We now describe the differences in beam definition between the rectangular segment and the square dot. While some minor caustic effects arise at the boundaries of the 5 $\mu$m-long segment, two clear beams radiate from the square dot, demonstrating the importance of a punctual source for the sharpness of the caustic beam. This also Bcomes clear when overlaying the Fourier transform of the excitation field distribution with the isofrequency curve as shown in Supplementary Fig. 1(a),(f). One can see the necessary condition of having the caustic point located within an effective region of the 2D emission spectrum in order to generate well-shaped beams.

Furthermore, a pronounced chiral coupling occurs in the DE configuration, for which no beam is observed on the left hand-side with respect to the bias field direction. This field-dependent non-reciprocity is essentially due to the non-negligible thickness/width aspect ratio of the stripline, which results in an out-of-plane microwave field distribution only favorable to single-sided propagating waves [5, 6]. In contrast, the caustic beams appear fully

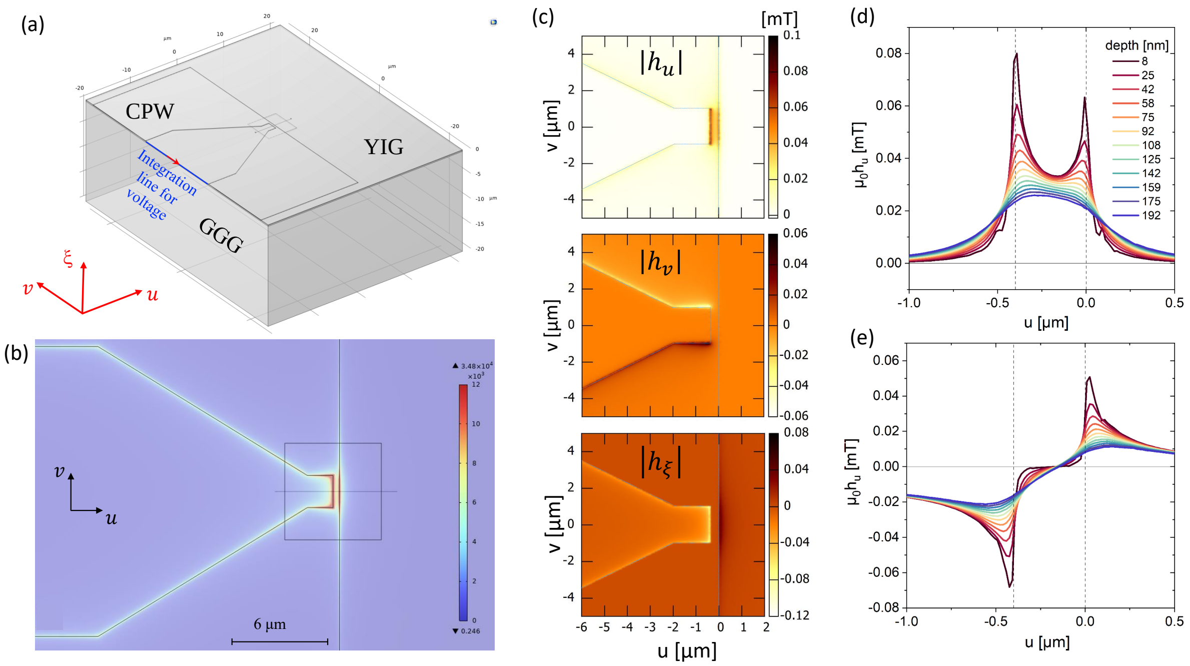


Supplementary Fig. 3. (**a**) Geometry of the 3D-layout used for the simulation. (**b**) Comsol simulation of the amplitude of the microwave field at 5 GHz around a 2 $\mu$m-long and 400 nm wide constriction. (**c**) Mapping of the three components of the microwave field around the constriction for the top cell. (**d**) Cross-section of $h_u$, and (**e**) $h_\xi$ in the middle of the constriction at different depth ranging through the whole 200 nm thickness of the YIG film.

symmetrical on either side of the bias field when it is parallel to the in-plane dynamic field.

## II. MICROWAVE FIELD DISTRIBUTION

To compare BLS measurements shown in Fig. 2 and Fig. 3 of the main article with MuMax and NFD simulations, we performed finite element simulations of the microwave field with Comsol Mutliphysics implementing the same GDS mask that was used to fabricate the 2 $\mu$m-long and 400 nm wide constriction device. These simulation results were then used as input for the both the NFD and micromagnetic simulations, normalizing the maximum value of the microwave field to 0.1 mT to ensure that the MuMax3 simulations were carried out in the linear regime.

We show in Supplementary Fig. 3(a) the 3D-layout, which consists of a coplanar waveguide (CPW) structure on top of a YIG/GGG sample within a total simulation volume of

40x40x40 $\mu m^3$. We adapted a progressive meshing with finer cell size for the region where the spatial variations are shorter, and ensured that further refining the cell size would not change the outcome of the simulation. To resolve this complex geometry, the mesh includes 1.2 million domain elements, 750,000 boundary elements, and 6,000 edge elements. These elements ensure accurate resolution of electromagnetic fields. Numeric-type ports are used with the Änalyze as a TEM fielöption to simulate the transverse electromagnetic mode, which is crucial for determining the characteristic impedance of the structure. Boundary mode analysis and the addition of a voltage integration line are required to calculate this impedance.

Supplementary Fig. 3(b) shows a mapping of the microwave field amplitude obtained at 5 GHz around a 2 $\mu$m-long and 400 nm wide constriction. We observe an inhomogeneous field distribution, with large spikes of intensity concentrated at the edges of the waveguide, which extend much further away from the constriction than one might intuitively anticipate, and which display an important $v$-component of the field at the angles of the constriction. We also show in Fig. 3(c)-(e) the evolution of the in-plane and out-of-plane components of the field in the depth of the 200 nm YIG film, and at the middle of the constriction ($v = 0$). Close to the top surface, we see somewhat unexpectidly that the in-plane component spikes at the lateral edges of the constriction over a few tens of nm, a lengthscale which is much smaller than the skin depth. These pinned concentrations of microwave power at the edges of the CPW may raise some questions regarding the actual field distribution of a real device. We anticipate that they could be an artefact of the simulations, for which the CPW structure is idealized with strictly right-angle corners, whereas a real device would most likely have rounded edges. Deeper in the YIG film, the field distribution becomes somewhat closer to the Oersted field produced by a straight conductor with rectangular section carrying uniformly distributed current. Although we cannot confirm the veracity of such an excitation profile in a real device, these results manifest the difficulty of assessing the microwave field distribution in sharp nanostructures.

## III. FULL SCALES MUMAX3 SIMULATIONS

We present in Supplementary Fig. 4 and Supplementary Fig. 5 the full-scale MuMax3 simulations shown respectively in Fig. 2 (DE-like configuration), and Fig. 3 (BVW-like con-

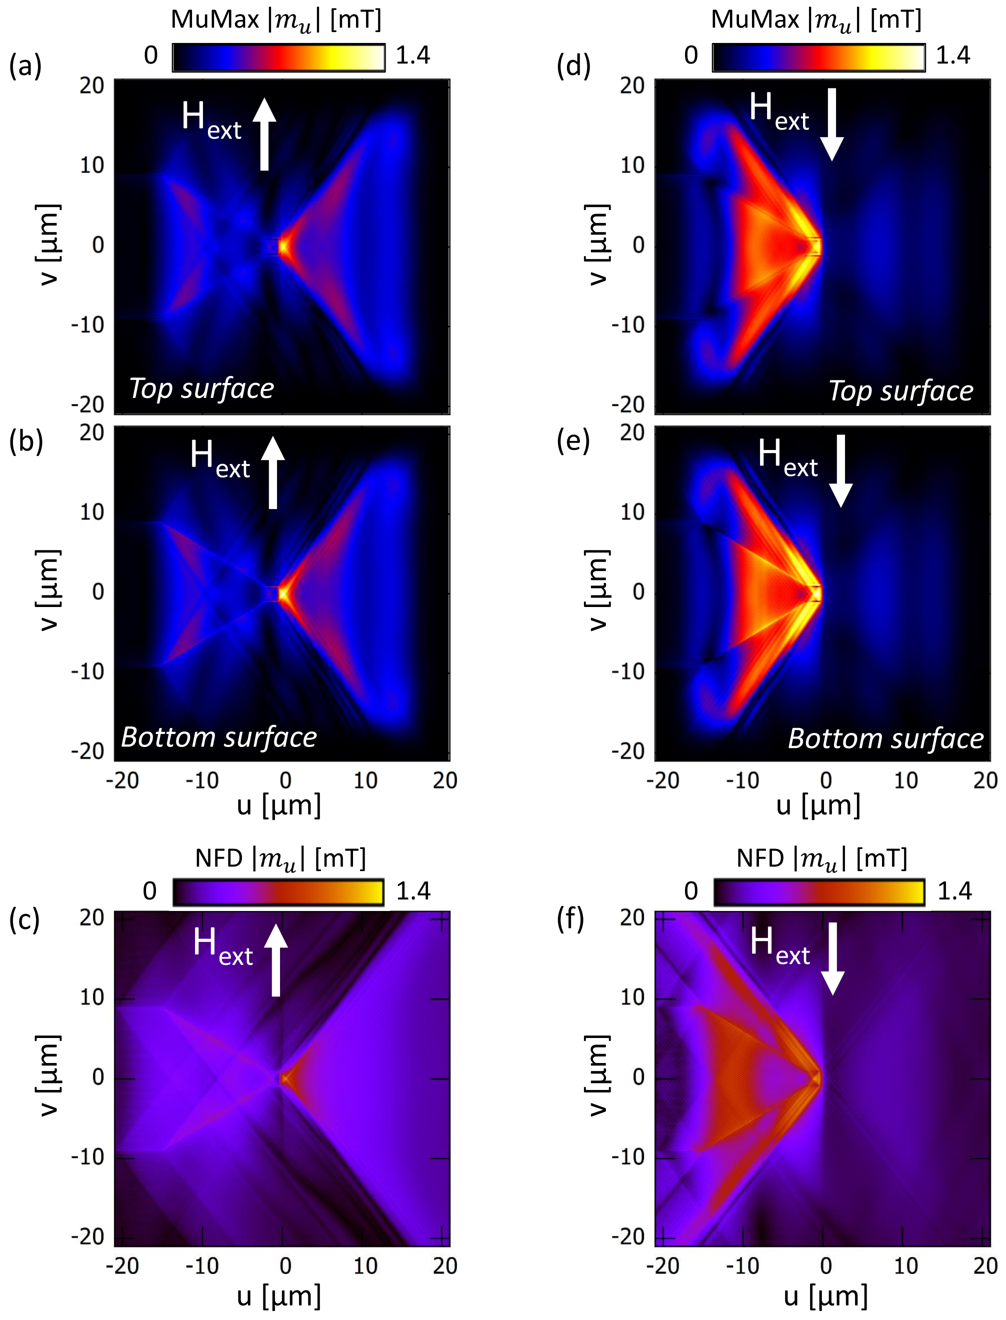


Supplementary Fig. 4. Full scale micromagnetic simulations at 7.5 GHz and +188mT of bias field applied along $v$ (DE) for (**a**) the top surface, and (**b**) the bottom surface. (**c**) Corresponding NFD simulation. (**d**),(**e**), and (**f**) are for -188mT.

figuration) of the main article, for which we used the field distribution obtained with Comsol to compare with the BLS measurements. We recall that the constriction is centered in $v = 0$, and that the right edge of the constriction is located at $u = 0$. We show both bias field

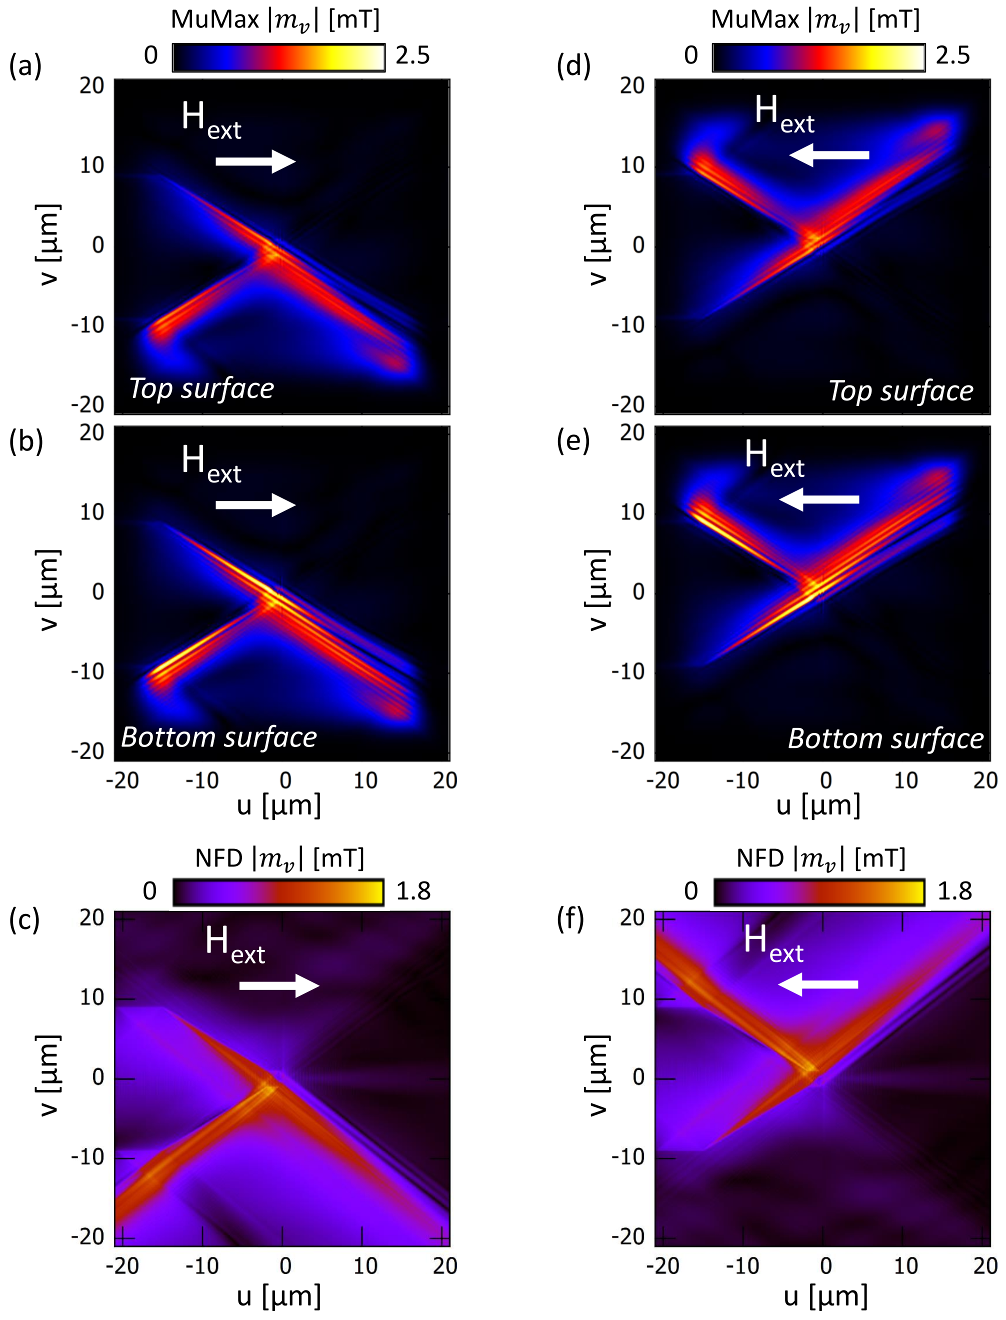


Supplementary Fig. 5. Full scale micromagnetic simulations at 7.5 GHz and +188mT of bias field applied along $u$ (BVW) for (**a**) the top surface, and (**b**) the bottom surface. (**c**) Corresponding NFD simulation. (**d**),(**e**), and (**f**) are for -188mT.

polarities, and compare spin-wave mapping for the top and bottom cell of the YIG film. We can see that the diffraction pattern does not change much between top and bottom surfaces. We see in particular that the chirality is very pronounced in the case of the negative bias

field (Supplementary Fig. 4(d),(e)), hardly any spin dynamics emerge on the right handside of the constriction.

Furthemore we systematically observe a larger amplitude for the bottom surface than for the top surface for both configurations, even though the field decays by a factor of  2 on average over the YIG thickness. This observation, which was already mentioned in the main text (Fig. 2-(h)), is due to the fact that chirality and mode localization work in opposite way for dipole-exchange spin-waves, namely chirality favors selectively spin-waves propagating towards the right hand-sides of the static magnetization direction, which also corresponds to a larger amplitude in the bottom surface. In other words, would the excitation originate from underneath the YIG film, this amplitude asymetry between top and bottom surfaces would be further enhanced due to the chiral coupling to the Oersted field.

We also show in Supplementary Fig. 4(c),(f) and Supplementary Fig. 5(c),(f) the corresponding NFD simulations on the same window size, for which we used a slightly larger cell size of 50 nm, and a full window size of 200 $\mu$m to allow for sufficient decay of the spin-wave and avoid any reflection on the edges of the window. Overall, the comparison between micromagnetic simulations and NFD is excellent, although some slight differences in the beam shape can be observed. These small discrepancies could be related to the possible higher order mode coupling which are taken into account in the NFD model.

## IV. FREQUENCY DEPENDENCE OF BEAM SHAPE - NFD SIMULATIONS

We present in Supplementary Fig. 6 (DE-like configuration), and Supplementary Fig. 7 (BVW-like configuration) large scale NFD simulations showing the frequency dependence of the beam formation at a bias field of 188 mT. We used the same color scale for each frequency. One can see that the frequency span over which the caustic beams are well-defined is fairly small, more or less 300 MHz, and that it is centered around the frequency / field values corresponding to FMR as was show in Fig. 4-(b) in the main article. Furthermore, the frequency span for which the caustic beam have the best shape differ between the DE-like and BVW-like configurations. While the beams are better defined sliglty before the FMR frequency (7.44 GHz) in the DE-like configuration, they appear better defined slightly after FMR in the BVW-like configuration. One can also follow the frequency dependence of the beam angle. It is essentially steered toward the bias field direction as the frequency

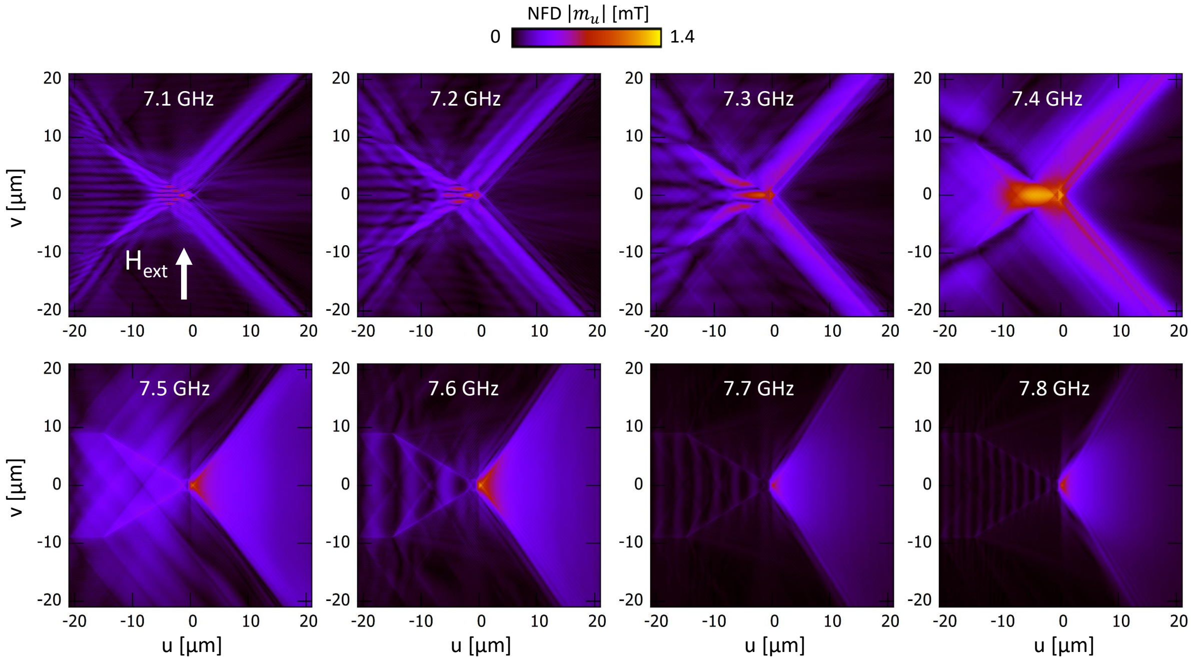


Supplementary Fig. 6. NFD simulations showing the evolution of the caustic beam with frequency for a +188mT bias field applied along $v$ (DE). FMR frequency is 7.44 GHz.

increases. However, in the BVW-like configuration, the beam angle at peak amplitude (Supplementary Fig. 7 at 7.5 GHz) differs slightly from predictions using the 2D-dispersion relation $f(k_u, k_v)$, as it was also observed experimentally in Fig. 4-(b) in the main article.

## V. BRILLOUIN LIGHT SCATTERING SPECTROSCOPY

We used microfocused Brillouin light scattering (BLS) spectroscopy in a back-scattering geometry using a continuous wavelength single-mode 532 nm wavelength laser at room temperature. A high-numerical-aperture (NA=0.75) objective lens collimates the scattered and reflected light within a large cone angle with respect to the sample surface normal. The optical resolution of the system is less than 500 nm. A light source is used to illuminate the sample for monitoring and controlling the measurement position. The inelastically scattered light is analyzed using a high-contrast multi-pass tandem Fabry Pérot interferometer with a contrast of at least $10^{15}$. The spin-wave signal is extracted from the Stokes peak. The acquisition time for a 5x30 $\mu m^2$ 2D spin-wave maps was approximately 48 hours for one

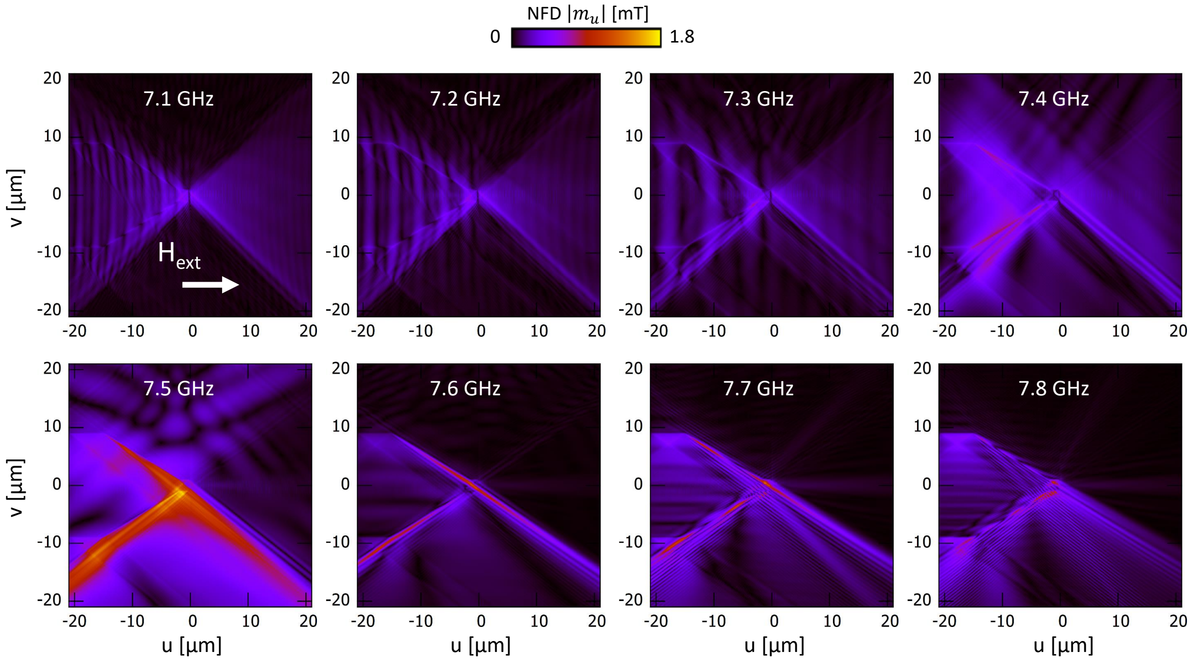


Supplementary Fig. 7. NFD simulations showing the evolution of the caustic beam with frequency for a +188mT bias field applied along $u$ (BVW). FMR frequency is 7.44 GHz.

field value. A BNC845 microwave source was used to excite the spin-wave caustics.

Supplmentary Figure 8 compares the 2D BLS maps where the recorded data is processed and normalized differently. (a) Unprocessed raw data without any processing. (b) 2D BLS intensity normalized to the reference peak of the laser, which is used to stabilize the interferometer. This is typically done to account for slow-varying changes in the environmental lab conditions. (c) 2D BLS intensity normalized by the maximum signal of the inelastically scattering light. (d) 2D BLS intensity normalized by both the reference signal and the maximum inelastically scattered light. (e) In addition to the processing shown in (d), the 2D BLS data is divided by the sum of the elements for each row, highlighting relative variations across the entire dataset. All experimental data shown in the main manuscript have been processed this way since the definition of the caustic is best presented using this method.

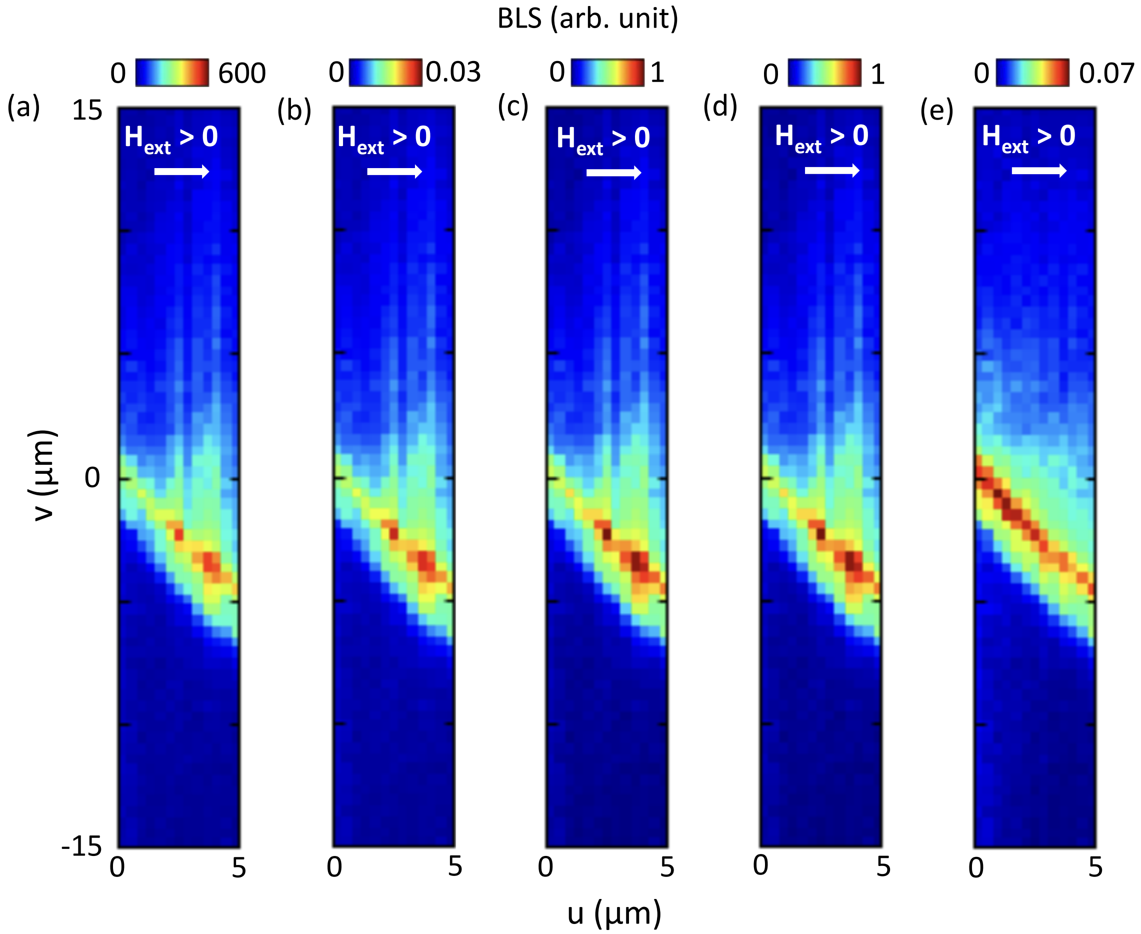


Supplementary Fig. 8. (a) Unprocessed raw data without any processing. (b) 2D BLS intensity normalized to the reference peak of the laser. (c) 2D BLS intensity normalized by the maximum signal of the inelastically scattering light. (d) 2D BLS intensity normalized by both the reference signal and the maximum inelastically scattered light. (e) 2D BLS data is divided by the sum of the elements for each row.

## VI. EXPERIMENTAL REALIZATION OF CAUSTIC SPIN WAVE

Different sizes of constrictions and different directions of the external bias field with respect to the microwave field direction were characterized by microfocused-BLS measurements on 200-nm thick YIG films.

Supplementary Fig. 9(a) shows the evolution of caustic angle for a constriction size $w = 400\ nm$ and $L = 2\ \mu m$ when the excitation frequency is slightly varied under the same external magnetic field of 188 mT applied along $+v$-direction, namely for excitation frequencies

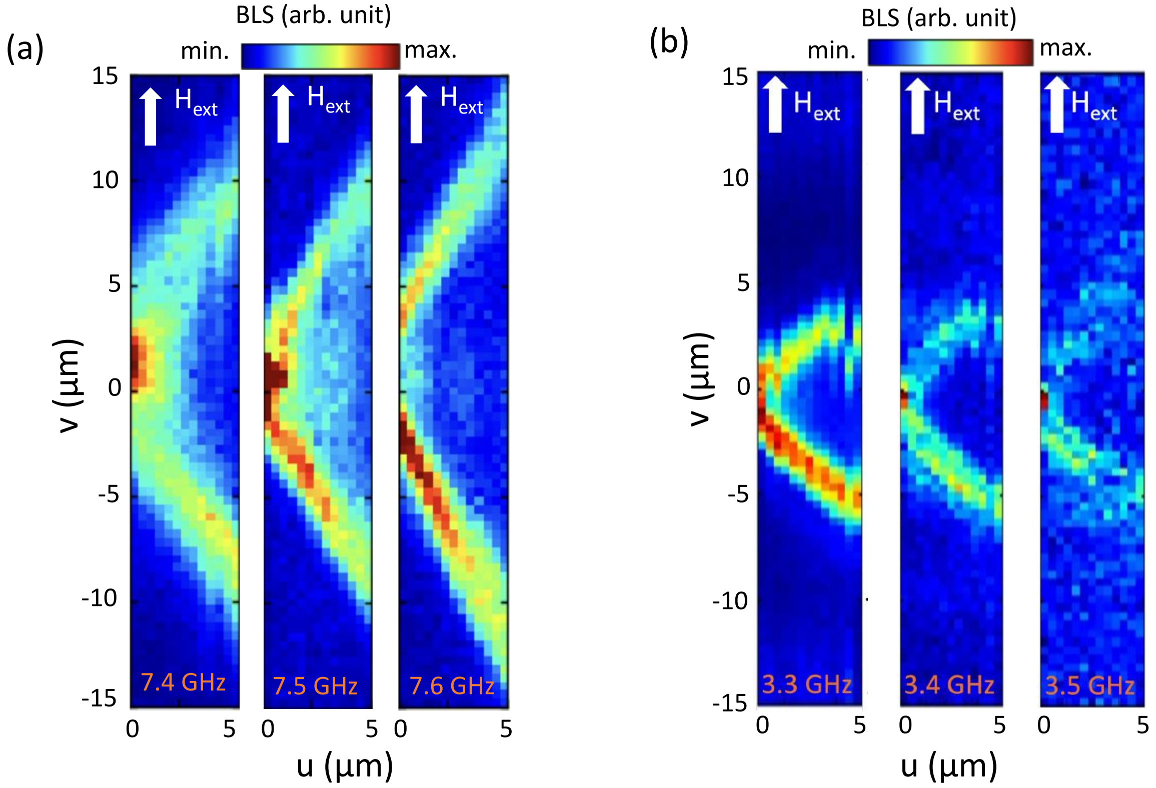


Supplementary Fig. 9. (**a**) BLS measurements showing the angular dependence of the caustic beam at a field of 188 mT and frequencies at 7.4 GHz, 7.5 GHz, and 7.6 GHz for a $w$=400 nm and $L$=2 $\mu$m constriction. (**b**) BLS measurement showing the angular dependence of the caustic beam at a field of 58 mT and frequencies at 3.3 GHz, 3.4 GHz, and 3.5 GHz for a $w$=200 nm and $L$=1 $\mu$m constriction.

of 7.4 GHz, 7.5 GHz, and 7.6 GHz. The middle panel of Supplementary Fig. 9 is identical to the one shown in Fig. 2(d) of the main manuscript. As is evident from the figure, the caustic angle increases with increasing frequency, in good agreement with the theoretical values obtained from the dispersion relation shown in Fig. 4(b) of the main manuscript. Supplementary Fig. **??**(b) shows the dependence of the caustic angle on the excitation frequency for a constriction of size $w = 200\ nm$ and $L = 1\ \mu m$ and an external bias field of 58 mT along the $+v$-direction. The excitation frequencies are 3.5 GHz, 3.4 GHz, and 3.3 GHz. The strongest signal was observed for a caustic beam excited at 3.3 GHz. The intensity decreased as the frequency increased, while the caustic angle remained approximately the same.

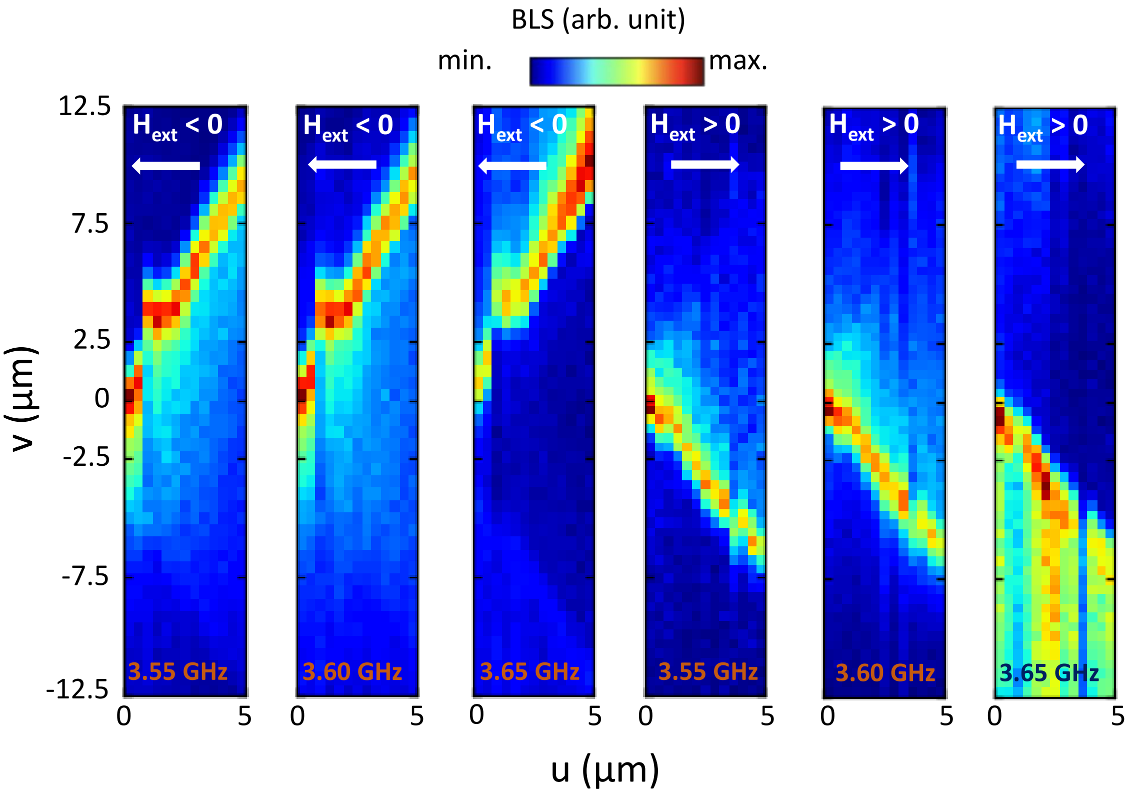


Supplementary Fig. 10. BLS measurements showing the angular dependence of the caustic beam at a field of ±67 mT and frequencies at 3.55 GHz, 3.60 GHz, and 3.65 GHz for a $w$=200 nm and $L$=1 $\mu$m constriction.

Finally, the corresponding frequency dependence of the caustic angle for a constriction of size $w = 200\ nm$ and $L = 1\ \mu m$ is shown in Supplementary Fig. 10. Here, the external bias field of 67 mT is applied along $-u$ and $+u$-directions, while the microwave frequencies was successively fixed to 3.55 GHz, 3.60 GHz, and 3.65 GHz.

## VII. FERROMAGNETIC RESONANCE CHARACTERIZATION OF YIG FILM

We use broadband ferromagnetic resonance (FMR) to determine the magnetic anisotropy, gyromagnetic ratio, and damping of the investigated 200-nm thick YIG film. Supplementary Fig. 11(a) shows the experimental FMR data obtained using a vector-network-analyzer-based FMR technique at room temperature. The experimental data is fitted using the

Kittel equation of the form:

$$f_{FMR} = \gamma' \mu_0 \sqrt{H(H + M_{eff})}, \tag{8}$$

where $\mu_0 = 4\pi \times 10^{-7}$ H/m is the permeability of free space, $\mu_0$M$_{eff}$ is the effective magnetization. From the fitting, we obtain $\mu_0$M$_{eff}$ = 187.2±6.3 mT and $\gamma'$ = 28.2±0.2 GHz/T. The corresponding value of the saturation magnetization obtained using vibrating sample magnetometry is 181.4 mT (not shown here), which is close to the value of effective magnetization obtained by FMR. This result suggests that any possible anisotropy in the film is negligible.

To determine the Gilbert damping parameter, we extracted the full-width half maximum of the FMR mode at different frequencies. The corresponding plot is shown in Supplementary Fig. 11(b). The effective Gilbert damping ($\alpha_{eff}$) is extracted using the linewidth equation:

$$\mu_0 \Delta H_{FWHM} = \mu_0 \Delta H_0 + \frac{2\alpha_{eff}}{\gamma\prime}, \tag{9}$$

where $\mu_0 \Delta H_0$ is the inhomogeneous linewidth. The extracted value is $\alpha_{eff}$ = 1.56× $10^{-4}$, which agrees well with comparable high-quality YIG films of this thickness. Here, we took into consideration the value of linewidth at ∼20 GHz and assumed the inhomogeneous linewidth broadening to be small (= 0 mT) to estimate the upper bound of effective Gilbert damping. The linewidths at lower frequencies were smaller than the field accuracy (1 Oe) and, hence, were omitted in the fitting process to extract the effective Gilbert damping parameter.

## VIII. BEAM ATTENUATION

In Supplementary Fig. 12(a), we present a 2D BLS map (60×80 $\mu$m$^2$) in the DE-like configuration at 7.5 GHz and 188 mT to study the long-range beam shaping and attenuation. As is obvious from the figure, the caustic beam propagates well over 100 $\mu$m, which is all the more remarkable considering the narrow constriction ($w$=400 nm, $L$=2 $\mu$m) from which it is emitted. Moreover, we observe a non-homogeneous decay of the beam: we observe 'pockets' of lower intensity reminiscent of a beating pattern. We also notice such inhomogeneities of the beam amplitude in the corresponding NFD simulation shown in Fig. 12(b), although they are not exactly located in the same locations as in the experiments. We attribute these

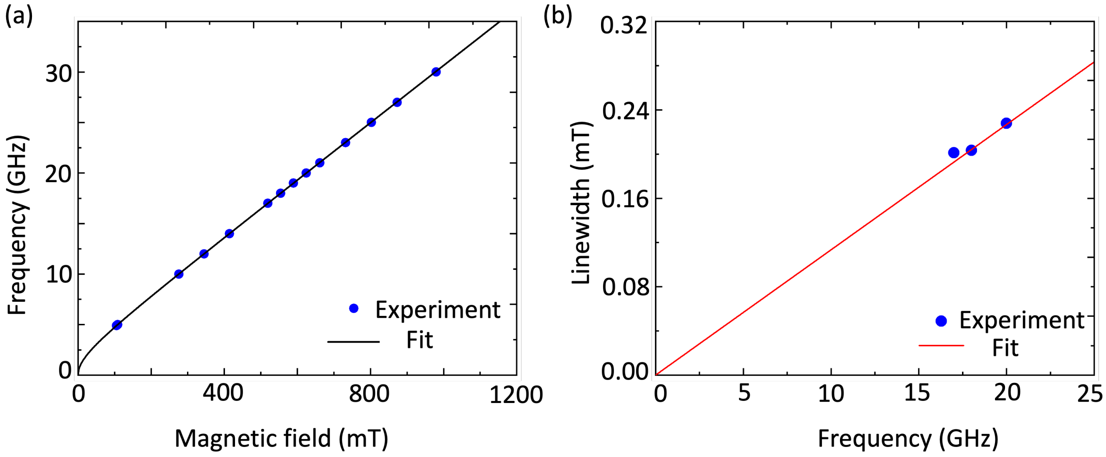


Supplementary Fig. 11. (**a**) Microwave frequency versus applied magnetic field for a 200-nm thick YIG film. Blue symbols show experimentally obtained broadband FMR data with the external field applied in the film plane. The back line is the resulting fit to the Kittel equation, Eq. (8). (**b**) Resonance linewidth versus applied microwave frequency. The blue symbols show the full-width half maximum value for different microwave frequencies; the red line is a fit using Eq. (9).

inhomogeneities of intensity along the caustic beam to some destructive interference between the different wavevectors composing the beam. On one hand, the finite range of wavevectors that meet the caustic condition $d^2k_y/dk_x^2 \sim 0$ have the same group velocity. However, they accumulate different phase delays throughout the propagation, leading inevitably to stationary wave patterns. Since the phase velocity and group velocity are close to orthogonal, interference lines approximately parallel to the beam propagation are formed, which are visible in all NFD simulations. On the other hand, the transition part of the antenna leading to the constriction also affects the overall beam shape due to the interference with the long-range spin waves emitted from the rest of the antenna. As can be seen from the NFD simulation of an isolated segment in Supplementary Fig. 2(g,i), the absence of such a transition to the constriction results in a finer definition of the beam.

Finally, we plot the amplitude evolution along the beam propagation in Supplementary Fig. 12(c) as extracted from (a). It shows an overall exponential decay with an effective attenuation length of about 45 $\mu$m, which is four times larger than the corresponding value for DE plane waves at the same field and wavevector values. The slower decay of caustic

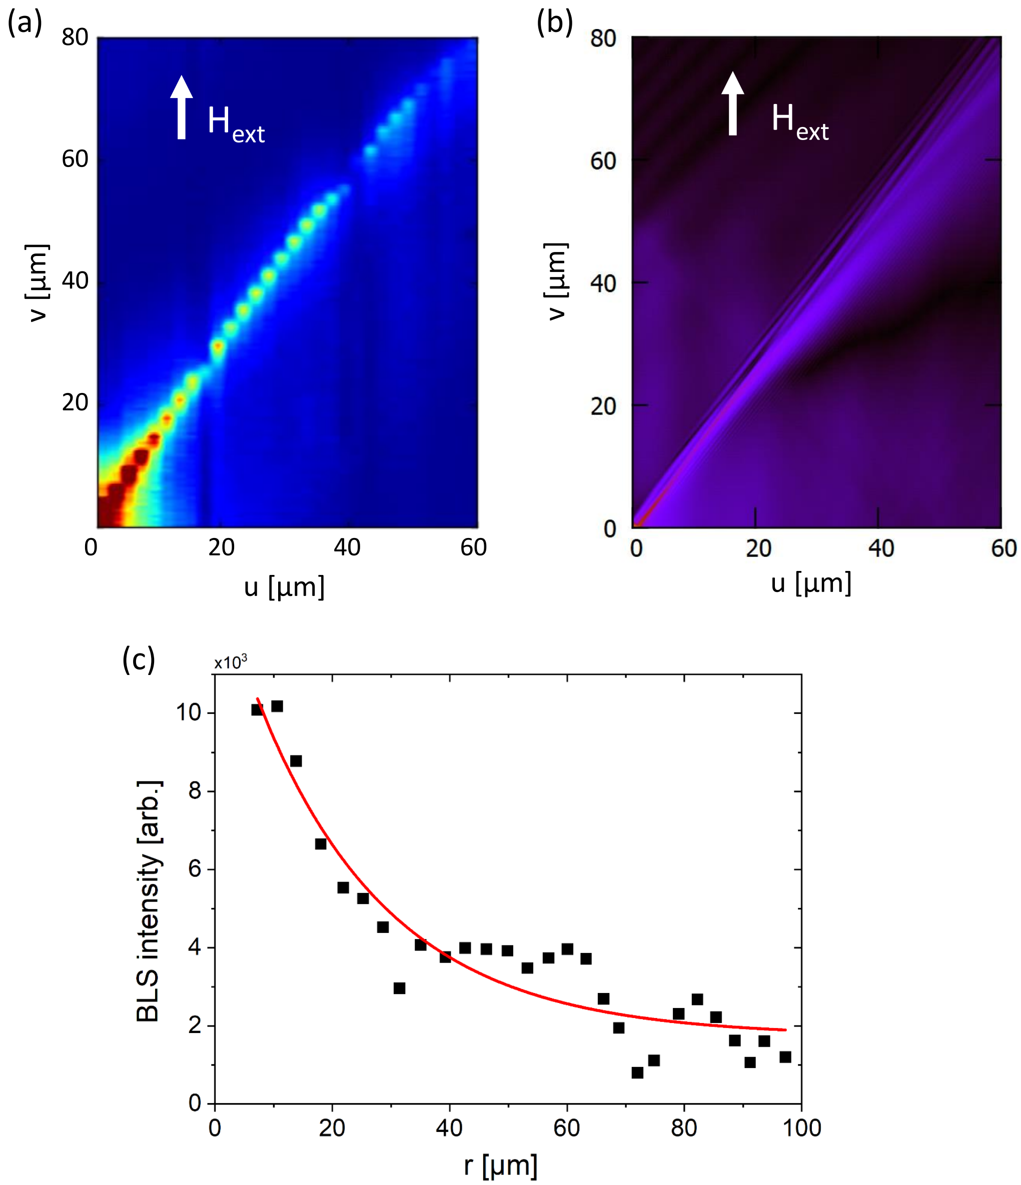


Supplementary Fig. 12. (**a**) Large-area BLS measurement at 7.5 GHz $\mu_0 H_{ext}$=+188 mT field in the Damon-Eshbach configuration for a 200 nm-wide and 2 $\mu$m-long constriction. (**b**) Corresponding NFD simulation. (**c**) Evolution of the caustic beam amplitude along its path extracted from (**a**).

beams appears as a strong asset for the development of magnonic devices.

---

[1] B. A. Kalinikos, Spectrum and linear excitation of spin waves in ferromagnetic films, Soviet Physics Journal **24**, 718 (1981).

[2] K. Y. Guslienko and A. N. Slavin, Magnetostatic green's functions for the description of spin waves in finite rectangular magnetic dots and stripes, Journal of Magnetism and Magnetic Materials **323**, 2418–2424 (2011).

[3] B. A. Kalinikos and A. N. Slavin, Theory of dipole-exchange spin wave spectrum for ferromagnetic films with mixed exchange boundary conditions, Journal of Physics C: Solid State Physics **19**, 7013 (1986).

[4] P. William H., B. P. Flannery, S. A. Teukolsky, and W. T. Vetterling, *Numerical Recipes in C* (Cambridge University Press, Cambridge, England, 1988).

[5] L. Temdie, V. Castel, C. Dubs, G. Pradhan, J. Solano, H. Majjad, R. Bernard, Y. Henry, M. Bailleul, and V. Vlaminck, High wave vector non-reciprocal spin wave beams, AIP Advances **13**, 025207 (2023).

[6] L. Temdie, V. Castel, T. Reimann, M. Lindner, C. Dubs, G. Pradhan, J. Solano, R. Bernard, H. Majjad, Y. Henry, M. Bailleul, and V. Vlaminck, Chiral excitation of exchange spin waves using gold nanowire grating, Magnetochemistry **9**, 199 (2023).
